# Supplementary material for: Analyzing Differentiable Fuzzy Implications
Source: arXiv:2006.03472 source file (2020-06-04)
Supplement: Supplementary file 1 [file appendix.tex]

In Machine Learning, the logistic function or sigmoid function $\sigma(x) = \frac{1}{1 + e^{-x}}$ is a common activation function \pcite{goodfellow2016deep}(p.65-66). This inspired \pcite{Sourek2018} to introduce parameterized families of aggregation functions they call Max-Sigmoid activation functions:

\begin{equation}
    A'_{\sigma +\wedge}(x_1, ..., x_n) = \sigma\left(s\cdot\left(\sum_{i=1}^n x_i - n + 1 + b_0\right)\right), \quad
    A'_{\sigma +\vee}(x_1, ..., x_n) = \sigma\left(s\cdot\left(\sum_{i=1}^n x_i + b_0\right)\right)
\end{equation}
We apply this transformation for any fuzzy implication $I: [0, 1]^2\rightarrow [0,1]$: 
\begin{equation}
    \sigma_I'(a, c) = \sigma(s\cdot(I(a, c) + b_0))
\end{equation}
This cannot be an aggregation function as $\sigma\in(0, 1)$ and so the boundary conditions $\sigma_I'(1, 1)=1$, $\sigma_I'(0, 0)=1$ and $\sigma_I'(1, 0)=0$ do not hold. We can solve this by adding two linear parameters $w$ and $h$, redefining $\sigma_I$ as
\begin{equation}
    \sigma_I(a, c) = w\cdot\sigma(s\cdot(I(a, c) + b_0)) - h
\end{equation}

For this, we need to make sure the lowest value of $I$ maps to 0 and the highest to 1: 
\begin{align}
   \label{eq:sigmaggis0}
   \sigma_I(1, 0) &= w\cdot\sigma(s\cdot(0 + b_0)) - h = 0 \\
   \label{eq:sigmaggis1}
   \sigma_I(1, 1) &= w\cdot\sigma(s\cdot(1 + b_0)) - h = 1
\end{align}

First solve both equations for $w$, starting with Equation \ref{eq:sigmaggis0}:

\begin{align}
    w\cdot\sigma(s\cdot b_0) - h &= 0 \notag \\
    \frac{1}{1+e^{-s\cdot b_0}} &= \frac{h}{w} \notag \\
    % 1 &= \frac{h}{w}\cdot(1 + e^{-s\cdot(inf_f + b_0)}) \notag \\
    % \frac{w}{h} &= 1 + e^{-s\cdot(inf_f + b_0)} \notag \\
    w &=  h\cdot (1 + e^{-s\cdot b_0})
    \label{eq:sigmeq2}
\end{align}
Likewise for Equation \ref{eq:sigmaggis1}:
\begin{align}
    w\cdot\sigma(s\cdot(1 + b_0)) - h &= 1 \notag \\
    \frac{1}{1+e^{-s\cdot(1 + b_0)}} &= \frac{1 + h}{w} \notag \\
    % 1 &= \frac{1+h}{w}\cdot(1 + e^{-s\cdot(sup_f + b_0)}) \notag \\
    % \frac{w}{1+h} &= 1 + e^{-s\cdot(sup_f + b_0)} \notag \\
    w &= (1 + h)\cdot (1 + e^{-s\cdot(1 + b_0)})
    \label{eq:sigmeq1}
\end{align}
Now we can solve for $h$ by equating Equations \ref{eq:sigmeq1} and \ref{eq:sigmeq2}. Then
\begin{align*}
    (1 + h)\cdot 1 + e^{-s\cdot(1 + b_0)} &=  h\cdot 1 + e^{-s\cdot b_0}\\
    h &= \frac{1 + e^{-s\cdot(1 + b_0)}}{1 + e^{-s\cdot b_0}-1 + e^{-s\cdot(1 + b_0)}}
\end{align*}
We thus get the following formula:
\begin{align}
    \sigma_I(a, c)
    %&= \frac{y_1}{y_2-y_1}\cdot y_2 \cdot \sigma\left(s\cdot\left(f(x_1, ..., x_n) + b_0\right)\right) - \frac{y_1}{y_2-y_1}\\
    &= \frac{1 + e^{-s\cdot(1 + b_0)}}{e^{-s\cdot b_0}-e^{-s\cdot(1 + b_0)}}\cdot \left(\left(1 + e^{-s\cdot b_0}\right) \cdot \sigma\left(s\cdot\left(I(a, c) + b_0\right)\right) - 1\right)
\end{align}

The most straightforward choice of $b_0$ is $-\frac{1}{2}$. This translates the outputs of $I$ to $[-\frac{1}{2}, \frac{1}{2}]$ and so it uses a symmetric part of the sigmoid function. With this value, we find the following simplification:
\begin{align}
        \sigma_{I}(a, c) &= \frac{1 + e^{-s (1-\frac{1}{2})}}{e^{s(0-\frac{1}{2})}-e^{-s(1-\frac{1}{2})}}\cdot \notag \\
  &\left(\left(1 + e^{-s(0-\frac{1}{2})}\right) \cdot \sigma\left(s\cdot\left(I(a, c) - \frac{1}{2}\right)\right) - 1\right) \\
  &= \frac{1 + e^{-\frac{s}{2}}}{e^{\frac{s}{2}}-e^{-\frac{s}{2}}}\cdot \frac{e^{\frac{s}{2}} - 1}{e^{\frac{s}{2}} - 1}\cdot 
  \left(\left(1 + e^{\frac{s}{2}}\right) \cdot \sigma\left(s\cdot\left(I(a, c) - \frac{1}{2}\right)\right) - 1\right) \\
  &= \frac{e^{\frac{s}{2}} - e^{-\frac{s}{2}}}{(e^{\frac{s}{2}}-e^{-\frac{s}{2}})(e^{\frac{s}{2}} - 1)}\cdot 
  \left(\left(1 + e^{\frac{s}{2}}\right) \cdot \sigma\left(s\cdot\left(I(a, c) - \frac{1}{2}\right)\right) - 1\right) \\
  &= \frac{1}{e^{\frac{s}{2}}-1}\cdot 
  \left(\left(1 + e^{\frac{s}{2}}\right) \cdot \sigma\left(s\cdot\left(I(a, c) - \frac{1}{2}\right)\right) - 1\right) \\
  &= \frac{\left(1 + e^{\frac{s}{2}}\right) \cdot \sigma\left(s\cdot I(a, c) - \frac{s}{2}\right) - 1}{e^{\frac{s}{2}}-1}
  \label{eq:deriv_sigmoid_tnorms}
%   &= \frac{1 + e^{-\frac{s}{2}}}{\left(e^{\frac{s}{2}} - 1\right)\cdot\left(1 + e^{-s\cdot\left(A_T(x_1, ..., x_n) - \frac{1}{2}\right)}\right)} - \frac{1}{e^{\frac{s}{2}} - 1} \\
%   &= \frac{e^{-\frac{s}{2}} - e^{-s\cdot\left(A_T(x_1, ..., x_n) - \frac{1}{2}\right)}}{\left(e^{\frac{s}{2}} - 1\right)\cdot\left(1 + e^{-s\cdot\left(A_T(x_1, ..., x_n) - \frac{1}{2}\right)}\right)}
\end{align}

Next, we proof several properties of the sigmoidal implication. 

\begin{prop}
\label{prop:sigm_mono_increase_f}
For all $a_1, c_1, a_2, c_2\in[0,1]$, 
\begin{enumerate}
    \item if $I(a_1, c_1) < I(a_2, c_2)$, then also $\sigma_I(a_1, c_1)< \sigma_I(a_2, c_2)$;
    \item if $I(a_1, c_1) = I(a_2, c_2)$, then also $\sigma_I(a_1, c_1)=\sigma_I(a_2, c_2)$.
\end{enumerate}
\end{prop}
\begin{proof}
\begin{enumerate}
\item We note that $\sigma_I$ can be written as $\sigma_I(a, c) = w\cdot \sigma\left(s\cdot\left(I(a, c) + \frac{1}{2}\right)\right) - h$ for constants $w=\frac{\left(1 + e^{-\frac{s}{2}}\right)^2}{e^{\frac{s}{2}}-e^{-\frac{s}{2}}}$ and $h=\frac{1 + e^{-\frac{s}{2}}}{e^{\frac{s}{2}}-e^{-\frac{s}{2}}}$. As $s>0$, $\frac{s}{2}>-\frac{s}{2}$. Therefore, $e^{\frac{s}{2}}-e^{-\frac{s}{2}}>0$. Furthermore, as $e^{-\frac{s}{2}} > 0$ then certainly $\left(1 + e^{-\frac{s}{2}}\right)^2 > 0$. As both $e^{\frac{s}{2}}-e^{-\frac{s}{2}}>0$ and $\left(1 + e^{-\frac{s}{2}}\right)^2>0$, then also $w>0$. As $s>0$, $s\cdot\left(I(a_1, c_1) + b_0\right) < s\cdot\left(I(a_2, c_2) + \frac{1}{2}\right)$ as by assumption $I(a_1, c_1) < I(a_2, c_2)$. Next, note that the sigmoid function $\sigma$ is a monotonically increasing function. Using $w>0$ we find that $\sigma_I(a_1, c_1) = w\cdot\sigma(s\cdot\left(I(a_1, c_1) + \frac{1}{2}\right)) < w\cdot\sigma(s\cdot\left(I(a_2, c_2) + \frac{1}{2}\right))=\sigma_I(a_2, c_2)$.
\item $$
    \sigma_I(a_1, c_1) = w\cdot \sigma\left(s\cdot\left(I(a_1, c_1) +\frac{1}{2}\right)\right) - h =  w\cdot \sigma\left(s\cdot\left(I(a_2, c_2) +\frac{1}{2}\right)\right) - h = \sigma_I(a_2, c_2) 
$$
\end{enumerate}
\end{proof}

\begin{prop}
\label{prop:sigm_supthenone}
$\sigma_I(a, c)$ is 1 if and only if $I(a, c) = 1$. Similarly, $\sigma_I(a, c)$ is 0 if and only if $I(a, c) = 0$. 
\end{prop}
\begin{proof}
Assume there is some $a, c\in[0, 1]$ so that $I(a, c) = 1$. By construction, $\sigma_I(a, c)$ is 1 (see \ref{appendix:sigm}).

Now assume there is some $a_1, c_1\in[0, 1]$ so that $\sigma_I(a_1,c_1) = 1$. Now consider some $a_2, c_2$ so that $I(a_2, c_2) = 1$. By the construction of $\sigma_I$, $\sigma_I(a_2, c_2) = 1$. For the sake of contradiction assume $I(a_1, c_1) < 1 $. However, by Proposition \ref{prop:sigm_mono_increase_f} as $I(a_1,c_1) < I(a_2,c_2)$ then $\sigma_I(a_1,c_1) < \sigma_I(a_2,c_2)$ has to hold. This is in contradiction with $\sigma_I(a_1, c_1) = \sigma_I(a_2, c_2) = 1$ so the assumption that $I(a_1, c_1)< 1$ has to be wrong and $I(a_1, c_1)=1$.

The proof for $I(a,c)=0$ is analogous.
\end{proof}

\begin{prop}
For all fuzzy implications $I$, $\sigma_I$ is also a fuzzy implication.
\end{prop}
\begin{proof}
By the definition of fuzzy implications, $I(\cdot, c)$ is decreasing and $I(a, \cdot)$ is increasing. Therefore, by Proposition \ref{prop:sigm_mono_increase_f}.1, $\sigma_I(\cdot, c)$ is also decreasing and $\sigma_I(a, \cdot)$ is also increasing. Furthermore, $I(0, 0) = 1$, $I(1, 1) = 1$ and $I(1, 0)=0$. We find by Proposition \ref{prop:sigm_supthenone} that then also $\sigma_I(0, 0) = 1$, $\sigma_I(1, 1) = 1$ and $\sigma_I(1, 0) = 0$. 
\end{proof}

$I$-sigmoidal implications only satisfy left-neutrality if $I$ is left-neutral and $s$ approaches 0.

\begin{prop}
\label{prop:sigm_contrapos}
If a fuzzy implication $I$ is contrapositive symmetric with respect to $N$, then $\sigma_I$ also is.% Similarly, if $I$ is left-contrapositive $\sigma_I$ is as well, and if $I$ is right-contrapositive $\sigma_I$ is too.
\end{prop}
\begin{proof}
Assume we have an implication $I$ that is contrapositive symmetric and so for all $a, c\in[0, 1]$, $I(a, c) = I(N(c), N(a))$. By Proposition \ref{prop:sigm_mono_increase_f}.2, $\sigma_I(a, c) = \sigma_I(N(c), N(a))$. Thus, $\sigma_I$ is also contrapositive symmetric with respect to $N$.
%The proofs for left- and right-contrapositive symmetry are similar.
\end{proof}
By this proposition, if $I$ is an S-implication, $\sigma_I$ is contrapositive symmetric and thus also contrapositive differentiable symmetric. 

\begin{prop}
If $I$ satisfies the identity principle, then $\sigma_I$ also satisfies the identity principle.
\end{prop}
\begin{proof}
Assume we have a fuzzy implication $I$ that satisfies the identity principle. Then $I(a, a) = 1$ for all $a$. By Proposition \ref{prop:sigm_supthenone} it holds that $\sigma_I(a, a)$ is also 1.
\end{proof}
